# Supplementary material for: Switchable band topology and geometric current in sliding bilayer elemental ferroelectric
Source: arXiv:2312.01937 source file (2023-12-04)
Supplement: Supplementary file 1 [file SI.pdf]

# Supplementary Material: Sliding-induced topological transition in bilayer bismuth

Zhuang Qian,<sup>1,2</sup> Zhihao Gong,<sup>3</sup> Jian Li,<sup>1,2</sup> Hua Wang,<sup>3,\*</sup> and Shi Liu<sup>1,2,†</sup>

*<sup>1</sup>Key Laboratory for Quantum Materials of Zhejiang Province,  
Department of Physics, School of Science and Research Center  
for Industries of the Future, Hangzhou Zhejiang 310030, China*

*<sup>2</sup>Institute of Natural Sciences, Westlake Institute for Advanced Study,  
Hangzhou, Zhejiang 310024, China*

*<sup>3</sup>ZJU-Hangzhou Global Scientific and Technological Innovation,  
School of Physics, Zhejiang University, Hangzhou 311215, China*

---

\* daodaohw@zju.edu.cn

† liushi@westlake.edu.cn

## I. COMPARING PBE+SOC AND HSE+SOC

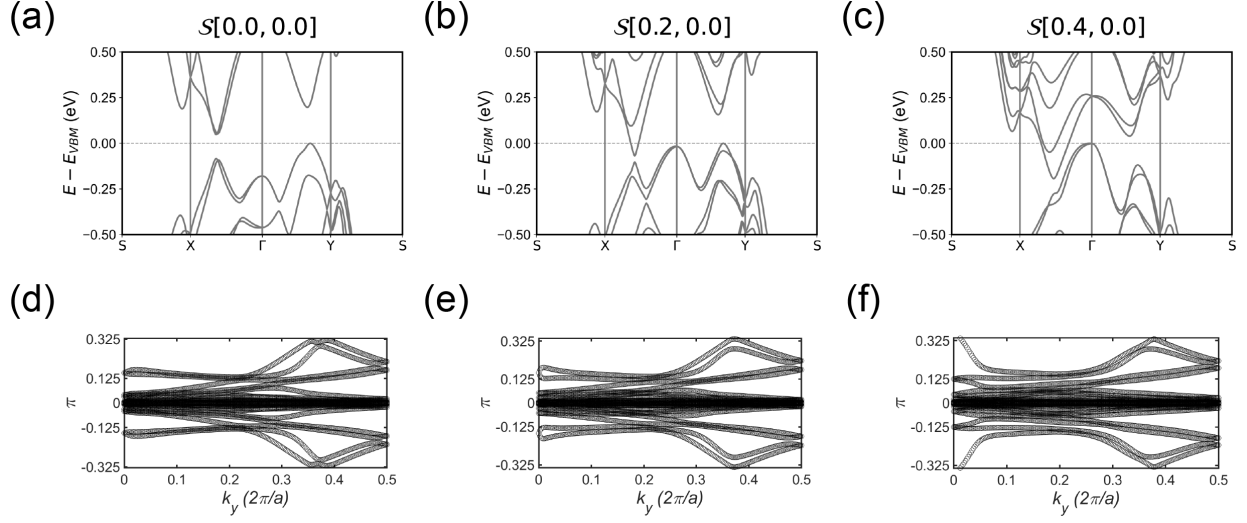

FIG. S1. PBE+SOC band structures for three configurations resulting from the sliding along the  $x$ -axis. The corresponding Wilson loop calculations are performed to analyze the topological properties of the band structures.

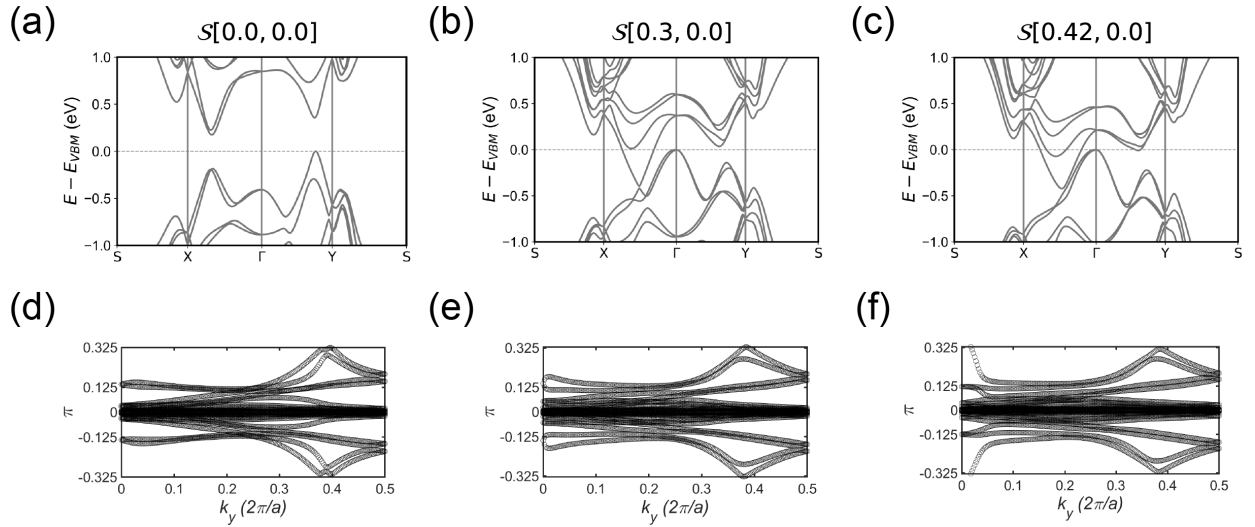

FIG. S2. HSE+SOC band structures and Wilson loop calculations for three configurations resulting from the sliding along the  $x$ -axis.
